# Supplementary material for: What Do Co-Folding Models Learn? Insights from Enhanced Transition Path Sampling
Source: arXiv:2611.30062 source file (2026-11-23)
Supplement: Supplementary file 1 [file si-labels.tex]

\newlabel{app:operations}{{S1}{2}{Sampling Algorithms}{section.1}{}}
\newlabel{app:operations@cref}{{[section][1][]S1}{[1][2][]2}}
\newlabel{app:prelim-ext}{{S1}{2}{Sampling Algorithms}{section.1}{}}
\newlabel{app:prelim-ext@cref}{{[section][1][]S1}{[1][2][]2}}
\newlabel{si:s1:gen}{{S1.1}{3}{The Boltz-2 Sampler}{subsection.1.1}{}}
\newlabel{si:s1:gen@cref}{{[subsection][1][1]S1.1}{[1][2][]3}}
\newlabel{eq:af3-schedule}{{S1}{3}{The Boltz-2 Sampler}{equation.S1}{}}
\newlabel{eq:af3-schedule@cref}{{[equation][1][]S1}{[1][2][]3}}
\newlabel{eq:af3-step}{{S2}{3}{The Boltz-2 Sampler}{equation.S2}{}}
\newlabel{eq:af3-step@cref}{{[equation][2][]S2}{[1][3][]3}}
\newlabel{eq:af3-step-full}{{S3}{3}{The Boltz-2 Sampler}{equation.S3}{}}
\newlabel{eq:af3-step-full@cref}{{[equation][3][]S3}{[1][3][]3}}
\newlabel{si:s1:base}{{S4}{3}{The Boltz-2 Sampler}{equation.S4}{}}
\newlabel{si:s1:base@cref}{{[equation][4][]S4}{[1][3][]3}}
\newlabel{si:s1:tps}{{S1.2}{3}{Transition Path Sampling}{subsection.1.2}{}}
\newlabel{si:s1:tps@cref}{{[subsection][2][1]S1.2}{[1][3][]3}}
\newlabel{si:s1:target}{{S5}{4}{Transition Path Sampling}{equation.S5}{}}
\newlabel{si:s1:target@cref}{{[equation][5][]S5}{[1][3][]4}}
\newlabel{eq:pcn}{{S6}{4}{Transition Path Sampling}{equation.S6}{}}
\newlabel{eq:pcn@cref}{{[equation][6][]S6}{[1][4][]4}}
\newlabel{si:s1:joint}{{S7}{4}{Transition Path Sampling}{equation.S7}{}}
\newlabel{si:s1:joint@cref}{{[equation][7][]S7}{[1][4][]4}}
\newlabel{si:s1:rev}{{S8}{4}{Transition Path Sampling}{equation.S8}{}}
\newlabel{si:s1:rev@cref}{{[equation][8][]S8}{[1][4][]4}}
\newlabel{si:s1:forward}{{S9}{4}{Transition Path Sampling}{equation.S9}{}}
\newlabel{si:s1:forward@cref}{{[equation][9][]S9}{[1][4][]4}}
\newlabel{alg:tps}{{S1}{5}{$\op {TPSstep}$. One shooting move of transition path sampling.\relax }{algorithm.S1}{}}
\newlabel{alg:tps@cref}{{[algorithm][1][]S1}{[1][5][]5}}
\newlabel{si:s1:reverse}{{S10}{5}{Transition Path Sampling}{equation.S10}{}}
\newlabel{si:s1:reverse@cref}{{[equation][10][]S10}{[1][4][]5}}
\newlabel{prop:mh-db}{{S11}{5}{Transition Path Sampling}{equation.S11}{}}
\newlabel{prop:mh-db@cref}{{[equation][11][]S11}{[1][5][]5}}
\newlabel{methods:sec:opes}{{S1.3}{5}{On-the-Fly Probability Enhanced Sampling}{subsection.1.3}{}}
\newlabel{methods:sec:opes@cref}{{[subsection][3][1]S1.3}{[1][5][]5}}
\newlabel{eq:opes-kde}{{S12}{6}{On-the-Fly Probability Enhanced Sampling}{equation.S12}{}}
\newlabel{eq:opes-kde@cref}{{[equation][12][]S12}{[1][6][]6}}
\newlabel{eq:opes-final}{{S13}{6}{On-the-Fly Probability Enhanced Sampling}{equation.S13}{}}
\newlabel{eq:opes-final@cref}{{[equation][13][]S13}{[1][6][]6}}
\newlabel{si:s1:explore}{{S14}{6}{On-the-Fly Probability Enhanced Sampling}{equation.S14}{}}
\newlabel{si:s1:explore@cref}{{[equation][14][]S14}{[1][6][]6}}
\newlabel{eq:rho-rm}{{S15}{6}{On-the-Fly Probability Enhanced Sampling}{equation.S15}{}}
\newlabel{eq:rho-rm@cref}{{[equation][15][]S15}{[1][6][]6}}
\newlabel{methods:sec:tempering}{{S1.4}{6}{Score Tempering and Replica Exchange}{subsection.1.4}{}}
\newlabel{methods:sec:tempering@cref}{{[subsection][4][1]S1.4}{[1][6][]6}}
\newlabel{alg:opes-deposit}{{S2}{7}{$\op {Deposit}$. One OPES deposit into the shared kernel bank.\relax }{algorithm.S2}{}}
\newlabel{alg:opes-deposit@cref}{{[algorithm][2][]S2}{[1][6][]7}}
\newlabel{alg:tps-opes}{{S3}{7}{TPS--OPES round. One round of TPS--OPES over the walkers of a bank.\relax }{algorithm.S3}{}}
\newlabel{alg:tps-opes@cref}{{[algorithm][3][]S3}{[1][6][]7}}
\newlabel{si:s1:step}{{S16}{7}{Tempered distribution and path weight}{equation.S16}{}}
\newlabel{si:s1:step@cref}{{[equation][16][]S16}{[1][7][]7}}
\newlabel{eq:prefix-velocity}{{S17}{8}{Tempered distribution and path weight}{equation.S17}{}}
\newlabel{eq:prefix-velocity@cref}{{[equation][17][]S17}{[1][7][]8}}
\newlabel{si:s1:ratio}{{S18}{8}{Tempered distribution and path weight}{equation.S18}{}}
\newlabel{si:s1:ratio@cref}{{[equation][18][]S18}{[1][8][]8}}
\newlabel{eq:score-w-final}{{S19}{8}{Tempered distribution and path weight}{equation.S19}{}}
\newlabel{eq:score-w-final@cref}{{[equation][19][]S19}{[1][8][]8}}
\newlabel{si:s1:mu}{{S20}{8}{Tempered distribution and path weight}{equation.S20}{}}
\newlabel{si:s1:mu@cref}{{[equation][20][]S20}{[1][8][]8}}
\newlabel{si:s1:bias}{{S21}{8}{Replica exchange}{equation.S21}{}}
\newlabel{si:s1:bias@cref}{{[equation][21][]S21}{[1][8][]8}}
\newlabel{si:s1:mt}{{S22}{8}{Replica exchange}{equation.S22}{}}
\newlabel{si:s1:mt@cref}{{[equation][22][]S22}{[1][8][]8}}
\newlabel{alg:score-temper}{{S4}{9}{$\op {ScoreTemperedSuffix}$. Regeneration of a path suffix on a tempered replica.\relax }{algorithm.S4}{}}
\newlabel{alg:score-temper@cref}{{[algorithm][4][]S4}{[1][9][]9}}
\newlabel{si:s1:offsets}{{S23}{9}{Replica exchange}{equation.S23}{}}
\newlabel{si:s1:offsets@cref}{{[equation][23][]S23}{[1][9][]9}}
\newlabel{def:replica-target}{{S24}{9}{Replica exchange}{equation.S24}{}}
\newlabel{def:replica-target@cref}{{[equation][24][]S24}{[1][9][]9}}
\newlabel{si:s1:ubase}{{S25}{10}{Replica exchange}{equation.S25}{}}
\newlabel{si:s1:ubase@cref}{{[equation][25][]S25}{[1][9][]10}}
\newlabel{si:s1:swap}{{S26}{10}{Replica exchange}{equation.S26}{}}
\newlabel{si:s1:swap@cref}{{[equation][26][]S26}{[1][10][]10}}
\newlabel{eq:delta-beta-Vij}{{S27}{10}{Replica exchange}{equation.S27}{}}
\newlabel{eq:delta-beta-Vij@cref}{{[equation][27][]S27}{[1][10][]10}}
\newlabel{eq:delta-logW}{{S28}{10}{Replica exchange}{equation.S28}{}}
\newlabel{eq:delta-logW@cref}{{[equation][28][]S28}{[1][10][]10}}
\newlabel{eq:swap-final}{{S29}{10}{Replica exchange}{equation.S29}{}}
\newlabel{eq:swap-final@cref}{{[equation][29][]S29}{[1][10][]10}}
\newlabel{si:s1:sign}{{S30}{10}{Replica exchange}{equation.S30}{}}
\newlabel{si:s1:sign@cref}{{[equation][30][]S30}{[1][10][]10}}
\newlabel{si:s1:halves}{{S31}{10}{Ladder spacing}{equation.S31}{}}
\newlabel{si:s1:halves@cref}{{[equation][31][]S31}{[1][10][]10}}
\newlabel{alg:replica-exchange}{{S5}{11}{Replica-exchange round. One replica-exchange round over the ladder.\relax }{algorithm.S5}{}}
\newlabel{alg:replica-exchange@cref}{{[algorithm][5][]S5}{[1][10][]11}}
\newlabel{si:s1:kl}{{S32}{11}{Ladder spacing}{equation.S32}{}}
\newlabel{si:s1:kl@cref}{{[equation][32][]S32}{[1][11][]11}}
\newlabel{eq:main-ladder-spacing}{{S33}{11}{Ladder spacing}{equation.S33}{}}
\newlabel{eq:main-ladder-spacing@cref}{{[equation][33][]S33}{[1][11][]11}}
\newlabel{si:s1:split}{{S34}{11}{Ladder spacing}{equation.S34}{}}
\newlabel{si:s1:split@cref}{{[equation][34][]S34}{[1][11][]11}}
\newlabel{methods:sec:landscape-reconstruction}{{S1.5}{12}{Landscape Reconstruction}{subsection.1.5}{}}
\newlabel{methods:sec:landscape-reconstruction@cref}{{[subsection][5][1]S1.5}{[1][11][]12}}
\newlabel{eq:logw-final}{{S35}{12}{Landscape Reconstruction}{equation.S35}{}}
\newlabel{eq:logw-final@cref}{{[equation][35][]S35}{[1][12][]12}}
\newlabel{eq:fes-state}{{S36}{12}{Landscape Reconstruction}{equation.S36}{}}
\newlabel{eq:fes-state@cref}{{[equation][36][]S36}{[1][12][]12}}
\newlabel{si:s1:state}{{S37}{12}{Landscape Reconstruction}{equation.S37}{}}
\newlabel{si:s1:state@cref}{{[equation][37][]S37}{[1][12][]12}}
\newlabel{eq:mbar}{{S38}{12}{Landscape Reconstruction}{equation.S38}{}}
\newlabel{eq:mbar@cref}{{[equation][38][]S38}{[1][12][]12}}
\newlabel{alg:fes-state-reweight}{{S6}{13}{$\op {ReconstructSurface}$. Reconstruction of the landscape from the recorded weights.\relax }{algorithm.S6}{}}
\newlabel{alg:fes-state-reweight@cref}{{[algorithm][6][]S6}{[1][12][]13}}
\newlabel{eq:fes}{{S39}{13}{Landscape Reconstruction}{equation.S39}{}}
\newlabel{eq:fes@cref}{{[equation][39][]S39}{[1][13][]13}}
\newlabel{app:methods-top}{{S2}{13}{Sampling Protocol}{section.2}{}}
\newlabel{app:methods-top@cref}{{[section][2][]S2}{[1][13][]13}}
\newlabel{methods:sampling-overview}{{S2}{13}{Sampling Protocol}{section.2}{}}
\newlabel{methods:sampling-overview@cref}{{[section][2][]S2}{[1][13][]13}}
\newlabel{sec:sampler}{{S2}{13}{Sampling Protocol}{section.2}{}}
\newlabel{sec:sampler@cref}{{[section][2][]S2}{[1][13][]13}}
\newlabel{methods:eftu-context}{{S2.1}{14}{System Preparation}{subsection.2.1}{}}
\newlabel{methods:eftu-context@cref}{{[subsection][1][2]S2.1}{[1][14][]14}}
\newlabel{app:tables}{{S2.1}{14}{System Preparation}{subsection.2.1}{}}
\newlabel{app:tables@cref}{{[subsection][1][2]S2.1}{[1][14][]14}}
\newlabel{app:matrix-tables}{{S2.1}{14}{System Preparation}{subsection.2.1}{}}
\newlabel{app:matrix-tables@cref}{{[subsection][1][2]S2.1}{[1][14][]14}}
\newlabel{tab:systems}{{S1}{15}{Campaign systems. Every cell uses the sampler shipped with its model (Algorithm~18 of AlphaFold~3, Section~\ref {app:prelim-ext}) at the official inference length of 200 steps, with three trunk recycles. The columns give the biased pair of collective variables $(s_1,s_2)$ (\Cref {app:cvs}) and the reference structure or state against which each variable is measured, where ``no reference'' marks a variable that is computed from the generated structure alone. The p38$\alpha $ and EF-Tu swing rows were added after the matrix.\relax }{table.caption.5}{}}
\newlabel{tab:systems@cref}{{[table][1][]S1}{[1][15][]15}}
\newlabel{si:protocol-ladder}{{S40}{17}{Composite Explore and Composite MetaD}{equation.S40}{}}
\newlabel{si:protocol-ladder@cref}{{[equation][40][]S40}{[1][17][]17}}
\newlabel{si:protocol-ladder-count}{{S41}{17}{Composite Explore and Composite MetaD}{equation.S41}{}}
\newlabel{si:protocol-ladder-count@cref}{{[equation][41][]S41}{[1][17][]17}}
\newlabel{tab:ladders}{{S2}{18}{Replica-exchange ladders and OPES barriers of every target. $d$ is three times the number of atoms, $\overline Q=73.3\,d$ the planned path quadratic (measured on chignolin and MAP2K1--FZC), and the replicas are the tempered replicas between $\gamma =1$ and $\gamma _{\mathrm {hot}}$ at $K_\star =1$ nat. Each ladder holds $148$ walkers ($296$ for the ternary complex), one per tempered replica and the remainder on the base replica. $\Delta E$ is the OPES barrier in kJ\,mol$^{-1}$ as set in the runs, where $250$, $40$ and $30$ are $59.8$, $9.6$ and $7.2$\,kcal\,mol$^{-1}$ ($\beta \Delta E\approx 100$, $16$ and $12$ at $k_{\mathrm B}T=0.596$\,kcal\,mol$^{-1}$). The three p38$\alpha $ systems of the two-site study reuse the ladder of 1a9u, and the Runs N' Poses complexes have a Composite MetaD cell only.\relax }{table.caption.6}{}}
\newlabel{tab:ladders@cref}{{[table][2][]S2}{[1][17][]18}}
\newlabel{app:cvs}{{S3}{18}{Collective Variables}{section.3}{}}
\newlabel{app:cvs@cref}{{[section][3][]S3}{[1][18][]18}}
\newlabel{eq:cv-distance}{{S42}{19}{Distances and RMSDs}{equation.S42}{}}
\newlabel{eq:cv-distance@cref}{{[equation][42][]S42}{[1][19][]19}}
\newlabel{eq:rmsd}{{S43}{19}{Distances and RMSDs}{equation.S43}{}}
\newlabel{eq:rmsd@cref}{{[equation][43][]S43}{[1][19][]19}}
\newlabel{si:cv-softmin}{{S44}{20}{Ligand and Pocket Variables}{equation.S44}{}}
\newlabel{si:cv-softmin@cref}{{[equation][44][]S44}{[1][20][]20}}
\newlabel{si:cv-softmin-excess}{{S45}{20}{Ligand and Pocket Variables}{equation.S45}{}}
\newlabel{si:cv-softmin-excess@cref}{{[equation][45][]S45}{[1][20][]20}}
\newlabel{eq:cv-pocket}{{S46}{20}{Ligand and Pocket Variables}{equation.S46}{}}
\newlabel{eq:cv-pocket@cref}{{[equation][46][]S46}{[1][20][]20}}
\newlabel{eq:rg}{{S47}{20}{Ligand and Pocket Variables}{equation.S47}{}}
\newlabel{eq:rg@cref}{{[equation][47][]S47}{[1][20][]20}}
\newlabel{eq:coord}{{S48}{20}{Ligand and Pocket Variables}{equation.S48}{}}
\newlabel{eq:coord@cref}{{[equation][48][]S48}{[1][20][]20}}
\newlabel{si:cv-switch}{{S49}{20}{Ligand and Pocket Variables}{equation.S49}{}}
\newlabel{si:cv-switch@cref}{{[equation][49][]S49}{[1][20][]20}}
\newlabel{si:cv-targets}{{S3.3}{20}{Definitions for Each Target}{subsection.3.3}{}}
\newlabel{si:cv-targets@cref}{{[subsection][3][3]S3.3}{[1][20][]20}}
\newlabel{app:methods}{{S4}{22}{Landscapes and States}{section.4}{}}
\newlabel{app:methods@cref}{{[section][4][]S4}{[1][22][]22}}
\newlabel{sec:metrics}{{S4.1}{22}{Landscape Estimation}{subsection.4.1}{}}
\newlabel{sec:metrics@cref}{{[subsection][1][4]S4.1}{[1][22][]22}}
\newlabel{tab:cvs}{{S3}{23}{Collective variables of each target. The symbols follow \cref {eq:cv-distance,eq:rmsd,eq:cv-pocket,eq:rg}, with the crystal as superscript, the measured set before the bar and the superposed set after the bar. Sets are C$\alpha $ atoms unless stated, and ``site'' is the backbone of the residues within $4\,\text {\AA }$ of the crystal ligand. The EF-Tu inputs with a ligand share one biased pair and are drawn on planes of their own.\relax }{table.caption.7}{}}
\newlabel{tab:cvs@cref}{{[table][3][]S3}{[1][22][]23}}
\newlabel{si:ana-snis}{{S50}{23}{Landscape Estimation}{equation.S50}{}}
\newlabel{si:ana-snis@cref}{{[equation][50][]S50}{[1][23][]23}}
\newlabel{si:ana-kish}{{S51}{23}{Landscape Estimation}{equation.S51}{}}
\newlabel{si:ana-kish@cref}{{[equation][51][]S51}{[1][23][]23}}
\newlabel{app:sampling-metrics}{{S4.2}{24}{Comparison Across Methods}{subsection.4.2}{}}
\newlabel{app:sampling-metrics@cref}{{[subsection][2][4]S4.2}{[1][24][]24}}
\newlabel{si:ana-grid-kernel}{{S52}{24}{Comparison Across Methods}{equation.S52}{}}
\newlabel{si:ana-grid-kernel@cref}{{[equation][52][]S52}{[1][24][]24}}
\newlabel{si:ana-neff}{{S53}{24}{Comparison Across Methods}{equation.S53}{}}
\newlabel{si:ana-neff@cref}{{[equation][53][]S53}{[1][24][]24}}
\newlabel{si:ana-bin-error}{{S54}{24}{Comparison Across Methods}{equation.S54}{}}
\newlabel{si:ana-bin-error@cref}{{[equation][54][]S54}{[1][24][]24}}
\newlabel{si:ana-score-step}{{S55}{25}{Comparison Across Methods}{equation.S55}{}}
\newlabel{si:ana-score-step@cref}{{[equation][55][]S55}{[1][25][]25}}
\newlabel{app:chances}{{S4.3}{25}{State Probabilities}{subsection.4.3}{}}
\newlabel{app:chances@cref}{{[subsection][3][4]S4.3}{[1][25][]25}}
\newlabel{eq:chance}{{S56}{25}{State Probabilities}{equation.S56}{}}
\newlabel{eq:chance@cref}{{[equation][56][]S56}{[1][25][]25}}
\newlabel{si:ana-chance-error}{{S57}{25}{State Probabilities}{equation.S57}{}}
\newlabel{si:ana-chance-error@cref}{{[equation][57][]S57}{[1][25][]25}}
\newlabel{si:ana-chance-grid}{{S58}{25}{State Probabilities}{equation.S58}{}}
\newlabel{si:ana-chance-grid@cref}{{[equation][58][]S58}{[1][25][]25}}
\newlabel{si:ana-basin-maps}{{S4.4}{26}{Basin Maps}{subsection.4.4}{}}
\newlabel{si:ana-basin-maps@cref}{{[subsection][4][4]S4.4}{[1][26][]26}}
\newlabel{app:states}{{S4.5}{26}{Identification of States}{subsection.4.5}{}}
\newlabel{app:states@cref}{{[subsection][5][4]S4.5}{[1][26][]26}}
\newlabel{app:case-figure-conventions}{{S4.5}{26}{Identification of States}{subsection.4.5}{}}
\newlabel{app:case-figure-conventions@cref}{{[subsection][5][4]S4.5}{[1][26][]26}}
\newlabel{si:ana-newton}{{S59}{26}{Identification of States}{equation.S59}{}}
\newlabel{si:ana-newton@cref}{{[equation][59][]S59}{[1][26][]26}}
\newlabel{si:ana-depth}{{S60}{26}{Identification of States}{equation.S60}{}}
\newlabel{si:ana-depth@cref}{{[equation][60][]S60}{[1][26][]26}}
\newlabel{si:ana-paths}{{S5}{27}{Minimum \texorpdfstring {$F_\theta $}{F} Paths}{section.5}{}}
\newlabel{si:ana-paths@cref}{{[section][5][]S5}{[1][27][]27}}
\newlabel{si:ana-string-method}{{S5.1}{27}{The Zero-Temperature String Method}{subsection.5.1}{}}
\newlabel{si:ana-string-method@cref}{{[subsection][1][5]S5.1}{[1][27][]27}}
\newlabel{si:ana-mep}{{S61}{27}{The Zero-Temperature String Method}{equation.S61}{}}
\newlabel{si:ana-mep@cref}{{[equation][61][]S61}{[1][27][]27}}
\newlabel{si:ana-string-steps}{{S5.2}{28}{Numerical Implementation}{subsection.5.2}{}}
\newlabel{si:ana-string-steps@cref}{{[subsection][2][5]S5.2}{[1][28][]28}}
\newlabel{si:ana-route-cost}{{S62}{28}{Numerical Implementation}{equation.S62}{}}
\newlabel{si:ana-route-cost@cref}{{[equation][62][]S62}{[1][28][]28}}
\newlabel{si:ana-string-step}{{S63}{28}{Numerical Implementation}{equation.S63}{}}
\newlabel{si:ana-string-step@cref}{{[equation][63][]S63}{[1][28][]28}}
\newlabel{si:ana-string-reparam}{{S64}{29}{Numerical Implementation}{equation.S64}{}}
\newlabel{si:ana-string-reparam@cref}{{[equation][64][]S64}{[1][29][]29}}
\newlabel{si:ana-string-ts}{{S5.3}{29}{Path Profiles and Transition States}{subsection.5.3}{}}
\newlabel{si:ana-string-ts@cref}{{[subsection][3][5]S5.3}{[1][29][]29}}
\newlabel{app:string-drag}{{S6}{30}{Adiabatic Mapping}{section.6}{}}
\newlabel{app:string-drag@cref}{{[section][6][]S6}{[1][30][]30}}
\newlabel{si:ana-drag-min}{{S6.1}{30}{Constrained Minimization}{subsection.6.1}{}}
\newlabel{si:ana-drag-min@cref}{{[subsection][1][6]S6.1}{[1][30][]30}}
\newlabel{si:ana-drag-kkt}{{S65}{30}{Constrained Minimization}{equation.S65}{}}
\newlabel{si:ana-drag-kkt@cref}{{[equation][65][]S65}{[1][30][]30}}
\newlabel{eq:string-drag}{{S66}{30}{Constrained Minimization}{equation.S66}{}}
\newlabel{eq:string-drag@cref}{{[equation][66][]S66}{[1][30][]30}}
\newlabel{si:ana-drag-gradient}{{S67}{30}{Constrained Minimization}{equation.S67}{}}
\newlabel{si:ana-drag-gradient@cref}{{[equation][67][]S67}{[1][30][]30}}
\newlabel{si:ana-drag-walk}{{S6.2}{31}{Hysteresis and Direction of Mapping}{subsection.6.2}{}}
\newlabel{si:ana-drag-walk@cref}{{[subsection][2][6]S6.2}{[1][31][]31}}
\newlabel{si:ana-delta-u}{{S68}{31}{Hysteresis and Direction of Mapping}{equation.S68}{}}
\newlabel{si:ana-delta-u@cref}{{[equation][68][]S68}{[1][31][]31}}
\newlabel{si:ana-drag-meaning}{{S6.3}{31}{Interpretation of the Mapped Energy}{subsection.6.3}{}}
\newlabel{si:ana-drag-meaning@cref}{{[subsection][3][6]S6.3}{[1][31][]31}}
\newlabel{si:ana-side-weight}{{S69}{32}{Interpretation of the Mapped Energy}{equation.S69}{}}
\newlabel{si:ana-side-weight@cref}{{[equation][69][]S69}{[1][32][]32}}
\newlabel{app:string-drag-exact}{{S6.4}{32}{Mapping Under the SuCOS Score}{subsection.6.4}{}}
\newlabel{app:string-drag-exact@cref}{{[subsection][4][6]S6.4}{[1][32][]32}}
\newlabel{si:ana-band-problem}{{S70}{32}{Mapping Under the SuCOS Score}{equation.S70}{}}
\newlabel{si:ana-band-problem@cref}{{[equation][70][]S70}{[1][32][]32}}
\newlabel{si:ana-score-linear}{{S71}{32}{Mapping Under the SuCOS Score}{equation.S71}{}}
\newlabel{si:ana-score-linear@cref}{{[equation][71][]S71}{[1][32][]32}}
\newlabel{si:ana-scores}{{S7}{33}{Exploration and Exploitation}{section.7}{}}
\newlabel{si:ana-scores@cref}{{[section][7][]S7}{[1][33][]33}}
\newlabel{si:ana-exploration}{{S7.1}{33}{Exploration Score}{subsection.7.1}{}}
\newlabel{si:ana-exploration@cref}{{[subsection][1][7]S7.1}{[1][33][]33}}
\newlabel{si:ana-compute}{{S72}{33}{Exploration Score}{equation.S72}{}}
\newlabel{si:ana-compute@cref}{{[equation][72][]S72}{[1][33][]33}}
\newlabel{si:ana-pooled}{{S73}{33}{Exploration Score}{equation.S73}{}}
\newlabel{si:ana-pooled@cref}{{[equation][73][]S73}{[1][33][]33}}
\newlabel{si:ana-pooled-surface}{{S74}{34}{Exploration Score}{equation.S74}{}}
\newlabel{si:ana-pooled-surface@cref}{{[equation][74][]S74}{[1][33][]34}}
\newlabel{eq:coverage}{{S75}{34}{Exploration Score}{equation.S75}{}}
\newlabel{eq:coverage@cref}{{[equation][75][]S75}{[1][34][]34}}
\newlabel{si:ana-exploitation}{{S7.2}{34}{Exploitation Score}{subsection.7.2}{}}
\newlabel{si:ana-exploitation@cref}{{[subsection][2][7]S7.2}{[1][34][]34}}
\newlabel{eq:fe-error}{{S76}{34}{Exploitation Score}{equation.S76}{}}
\newlabel{eq:fe-error@cref}{{[equation][76][]S76}{[1][34][]34}}
\newlabel{si:ana-offset}{{S77}{34}{Exploitation Score}{equation.S77}{}}
\newlabel{si:ana-offset@cref}{{[equation][77][]S77}{[1][34][]34}}
\newlabel{si:diagnostics}{{S8}{35}{Structural Diagnostics}{section.8}{}}
\newlabel{si:diagnostics@cref}{{[section][8][]S8}{[1][35][]35}}
\newlabel{si:diag-eftu}{{S8.1}{35}{Structural Analysis of EF-Tu}{subsection.8.1}{}}
\newlabel{si:diag-eftu@cref}{{[subsection][1][8]S8.1}{[1][35][]35}}
\newlabel{si:eftu-turn-angle}{{S78}{35}{Structural Analysis of EF-Tu}{equation.S78}{}}
\newlabel{si:eftu-turn-angle@cref}{{[equation][78][]S78}{[1][35][]35}}
\newlabel{si:diag-amber}{{S8.2}{36}{Steric Overlaps and Ligand Stereochemistry}{subsection.8.2}{}}
\newlabel{si:diag-amber@cref}{{[subsection][2][8]S8.2}{[1][36][]36}}
\newlabel{si:diag-handedness}{{S8.2}{36}{Steric Overlaps and Ligand Stereochemistry}{subsection.8.2}{}}
\newlabel{si:diag-handedness@cref}{{[subsection][2][8]S8.2}{[1][36][]36}}
\newlabel{si:amber-signed-volume}{{S79}{36}{Steric Overlaps and Ligand Stereochemistry}{equation.S79}{}}
\newlabel{si:amber-signed-volume@cref}{{[equation][79][]S79}{[1][36][]36}}
\newlabel{app:experiment}{{S9}{37}{Comparison with Experiment and Training Data}{section.9}{}}
\newlabel{app:experiment@cref}{{[section][9][]S9}{[1][37][]37}}
\newlabel{si:exp-rmsf}{{S80}{37}{Comparison with Experiment and Training Data}{equation.S80}{}}
\newlabel{si:exp-rmsf@cref}{{[equation][80][]S80}{[1][37][]37}}
\newlabel{si:exp-rmsf-moments}{{S81}{37}{Comparison with Experiment and Training Data}{equation.S81}{}}
\newlabel{si:exp-rmsf-moments@cref}{{[equation][81][]S81}{[1][37][]37}}
\newlabel{si:exp-src-direction}{{S82}{38}{Comparison with Experiment and Training Data}{equation.S82}{}}
\newlabel{si:exp-src-direction@cref}{{[equation][82][]S82}{[1][38][]38}}
\newlabel{si:methods-validation}{{S10}{39}{Validation and Reproducibility}{section.10}{}}
\newlabel{si:methods-validation@cref}{{[section][10][]S10}{[1][38][]39}}
\newlabel{methods:toy-validation}{{S10.1}{39}{Analytic Double-Well Model}{subsection.10.1}{}}
\newlabel{methods:toy-validation@cref}{{[subsection][1][10]S10.1}{[1][39][]39}}
\newlabel{si:toy-score}{{S83}{39}{Analytic Double-Well Model}{equation.S83}{}}
\newlabel{si:toy-score@cref}{{[equation][83][]S83}{[1][39][]39}}
\newlabel{methods:reproducibility}{{S10.2}{39}{Reproducibility and Use of AI Tools}{subsection.10.2}{}}
\newlabel{methods:reproducibility@cref}{{[subsection][2][10]S10.2}{[1][39][]39}}
\newlabel{methods:ai-tools}{{S10.2}{39}{Reproducibility and Use of AI Tools}{subsection.10.2}{}}
\newlabel{methods:ai-tools@cref}{{[subsection][2][10]S10.2}{[1][39][]39}}
\newlabel{tab:resources}{{S4}{40}{Software and data used in this study.\relax }{table.caption.8}{}}
\newlabel{tab:resources@cref}{{[table][4][]S4}{[1][40][]40}}
\newlabel{app:proofs}{{S11}{40}{Theoretical Derivations}{section.11}{}}
\newlabel{app:proofs@cref}{{[section][11][]S11}{[1][40][]40}}
\newlabel{app:stationarity}{{S11.1}{40}{Stationarity of the Sampler}{subsection.11.1}{}}
\newlabel{app:stationarity@cref}{{[subsection][1][11]S11.1}{[1][40][]40}}
\newlabel{app:proof-tps}{{S11.1}{41}{Reversibility of the shooting move}{section*.9}{}}
\newlabel{app:proof-tps@cref}{{[subsection][1][11]S11.1}{[1][40][]41}}
\newlabel{si:exact-pair-symmetric}{{S84}{41}{Reversibility of the shooting move}{equation.S84}{}}
\newlabel{si:exact-pair-symmetric@cref}{{[equation][84][]S84}{[1][41][]41}}
\newlabel{si:exact-pcn-reversible}{{S85}{41}{Reversibility of the shooting move}{equation.S85}{}}
\newlabel{si:exact-pcn-reversible@cref}{{[equation][85][]S85}{[1][41][]41}}
\newlabel{si:exact-mh-fixed-k}{{S86}{41}{Reversibility of the shooting move}{equation.S86}{}}
\newlabel{si:exact-mh-fixed-k@cref}{{[equation][86][]S86}{[1][41][]41}}
\newlabel{si:exact-walker-mixture}{{S87}{41}{Reversibility of the shooting move}{equation.S87}{}}
\newlabel{si:exact-walker-mixture@cref}{{[equation][87][]S87}{[1][41][]41}}
\newlabel{app:proof-temper}{{S11.1}{42}{Tempered path weight}{section*.10}{}}
\newlabel{app:proof-temper@cref}{{[subsection][1][11]S11.1}{[1][41][]42}}
\newlabel{si:exact-step-ratio}{{S88}{42}{Tempered path weight}{equation.S88}{}}
\newlabel{si:exact-step-ratio@cref}{{[equation][88][]S88}{[1][42][]42}}
\newlabel{si:exact-step-bracket}{{S89}{42}{Tempered path weight}{equation.S89}{}}
\newlabel{si:exact-step-bracket@cref}{{[equation][89][]S89}{[1][42][]42}}
\newlabel{si:exact-path-weight-sum}{{S90}{42}{Tempered path weight}{equation.S90}{}}
\newlabel{si:exact-path-weight-sum@cref}{{[equation][90][]S90}{[1][42][]42}}
\newlabel{app:proof-pt-stationarity}{{S11.1}{42}{Replica exchange}{section*.11}{}}
\newlabel{app:proof-pt-stationarity@cref}{{[subsection][1][11]S11.1}{[1][42][]42}}
\newlabel{si:exact-swap-ratio}{{S91}{42}{Replica exchange}{equation.S91}{}}
\newlabel{si:exact-swap-ratio@cref}{{[equation][91][]S91}{[1][42][]42}}
\newlabel{si:exact-swap-mu}{{S92}{43}{Replica exchange}{equation.S92}{}}
\newlabel{si:exact-swap-mu@cref}{{[equation][92][]S92}{[1][42][]43}}
\newlabel{si:exact-reweighting}{{S11.1}{43}{Reweighting identities}{section*.12}{}}
\newlabel{si:exact-reweighting@cref}{{[subsection][1][11]S11.1}{[1][43][]43}}
\newlabel{si:exact-snis}{{S93}{43}{Reweighting identities}{equation.S93}{}}
\newlabel{si:exact-snis@cref}{{[equation][93][]S93}{[1][43][]43}}
\newlabel{si:exact-label-probability}{{S94}{43}{Reweighting identities}{equation.S94}{}}
\newlabel{si:exact-label-probability@cref}{{[equation][94][]S94}{[1][43][]43}}
\newlabel{si:exact-mbar-stationarity}{{S95}{43}{Reweighting identities}{equation.S95}{}}
\newlabel{si:exact-mbar-stationarity@cref}{{[equation][95][]S95}{[1][43][]43}}
\newlabel{si:exact-ess-window}{{S96}{44}{Reweighting identities}{equation.S96}{}}
\newlabel{si:exact-ess-window@cref}{{[equation][96][]S96}{[1][44][]44}}
\newlabel{app:scaling-derivations}{{S11.2}{44}{Scaling Laws for the Coverage and Exploitation Error}{subsection.11.2}{}}
\newlabel{app:scaling-derivations@cref}{{[subsection][2][11]S11.2}{[1][44][]44}}
\newlabel{eq:main-coverage-walk}{{S97}{44}{Scaling Laws for the Coverage and Exploitation Error}{equation.S97}{}}
\newlabel{eq:main-coverage-walk@cref}{{[equation][97][]S97}{[1][44][]44}}
\newlabel{si:walk-coverage-iid}{{S11.2}{45}{Independent sampling}{section*.13}{}}
\newlabel{si:walk-coverage-iid@cref}{{[subsection][2][11]S11.2}{[1][44][]45}}
\newlabel{eq:main-gumbel}{{S98}{45}{Independent sampling}{equation.S98}{}}
\newlabel{eq:main-gumbel@cref}{{[equation][98][]S98}{[1][45][]45}}
\newlabel{si:walk-coverage-sum}{{S99}{45}{Independent sampling}{equation.S99}{}}
\newlabel{si:walk-coverage-sum@cref}{{[equation][99][]S99}{[1][45][]45}}
\newlabel{si:walk-coverage-indicator}{{S100}{45}{Independent sampling}{equation.S100}{}}
\newlabel{si:walk-coverage-indicator@cref}{{[equation][100][]S100}{[1][45][]45}}
\newlabel{eq:coverage-law}{{S101}{45}{Independent sampling}{equation.S101}{}}
\newlabel{eq:coverage-law@cref}{{[equation][101][]S101}{[1][45][]45}}
\newlabel{eq:exponent-exact}{{S102}{45}{Independent sampling}{equation.S102}{}}
\newlabel{eq:exponent-exact@cref}{{[equation][102][]S102}{[1][45][]45}}
\newlabel{si:walk-coverage-powerlaw}{{S103}{45}{Independent sampling}{equation.S103}{}}
\newlabel{si:walk-coverage-powerlaw@cref}{{[equation][103][]S103}{[1][45][]45}}
\newlabel{fig:coverage-law}{{S1}{46}{Coverage law of independent generation. For each target, the coverage of the independent cell against rounds on logarithmic axes (green; dots mark measured points) and the coverage law of \cref {eq:coverage-law} (black, dashed), which takes the probability $p_b$ of each support bin from the pooled landscape, with no free parameter. The gray guide marks the slope $t^{0.2}$. The law predicts the measured curve to within $3\%$ on the five targets with broad maps, whereas on chignolin and on the two p38$\alpha $ inputs with 4-FPP the measured curve rises above the law at late rounds.\relax }{figure.caption.14}{}}
\newlabel{fig:coverage-law@cref}{{[figure][1][]S1}{[1][45][]46}}
\newlabel{eq:main-exponent}{{S104}{46}{Independent sampling}{equation.S104}{}}
\newlabel{eq:main-exponent@cref}{{[equation][104][]S104}{[1][45][]46}}
\newlabel{si:walk-coverage-biased}{{S11.2}{46}{Biased sampling}{section*.15}{}}
\newlabel{si:walk-coverage-biased@cref}{{[subsection][2][11]S11.2}{[1][46][]46}}
\newlabel{si:walk-biased-density}{{S105}{47}{Biased sampling}{equation.S105}{}}
\newlabel{si:walk-biased-density@cref}{{[equation][105][]S105}{[1][46][]47}}
\newlabel{si:walk-height-step-exact}{{S106}{47}{Biased sampling}{equation.S106}{}}
\newlabel{si:walk-height-step-exact@cref}{{[equation][106][]S106}{[1][47][]47}}
\newlabel{eq:main-height-step}{{S107}{47}{Biased sampling}{equation.S107}{}}
\newlabel{eq:main-height-step@cref}{{[equation][107][]S107}{[1][47][]47}}
\newlabel{eq:main-height-fp}{{S108}{47}{Biased sampling}{equation.S108}{}}
\newlabel{eq:main-height-fp@cref}{{[equation][108][]S108}{[1][47][]47}}
\newlabel{fig:height-diffusion}{{S2}{48}{Height diffusion under a flattening bias. (A)~Filled height $L=\nu ^{-1}(C)$ against rounds for the four targets with broad maps, with the mean height of the walk of \cref {eq:main-height-fp} at $D_u=0.3$ (dashed) and the Gaussian model of the shooting move without fitting (dotted). (B)~Coverage exponents over rounds $10$--$70$ for the same samples counted along one biased CV, along both, and along both plus an unbiased CV, with medians over cells as bars and $d_s/4$ dashed.\relax }{figure.caption.16}{}}
\newlabel{fig:height-diffusion@cref}{{[figure][2][]S2}{[1][47][]48}}
\newlabel{si:walk-half-gaussian}{{S109}{48}{Biased sampling}{equation.S109}{}}
\newlabel{si:walk-half-gaussian@cref}{{[equation][109][]S109}{[1][47][]48}}
\newlabel{eq:main-exponent-kinetic}{{S110}{48}{Biased sampling}{equation.S110}{}}
\newlabel{eq:main-exponent-kinetic@cref}{{[equation][110][]S110}{[1][48][]48}}
\newlabel{si:walk-error}{{S11.2}{49}{Landscape error}{section*.17}{}}
\newlabel{si:walk-error@cref}{{[subsection][2][11]S11.2}{[1][49][]49}}
\newlabel{si:walk-error-law}{{S111}{49}{Landscape error}{equation.S111}{}}
\newlabel{si:walk-error-law@cref}{{[equation][111][]S111}{[1][49][]49}}
\newlabel{eq:main-memory-time}{{S112}{49}{Landscape error}{equation.S112}{}}
\newlabel{eq:main-memory-time@cref}{{[equation][112][]S112}{[1][49][]49}}
\newlabel{si:walk-occupation}{{S11.2}{50}{First-passage statistics}{section*.18}{}}
\newlabel{si:walk-occupation@cref}{{[subsection][2][11]S11.2}{[1][49][]50}}
\newlabel{eq:renewal-moments}{{S113}{50}{First-passage statistics}{equation.S113}{}}
\newlabel{eq:renewal-moments@cref}{{[equation][113][]S113}{[1][50][]50}}
\newlabel{eq:occupation-variance}{{S114}{50}{First-passage statistics}{equation.S114}{}}
\newlabel{eq:occupation-variance@cref}{{[equation][114][]S114}{[1][50][]50}}
\newlabel{eq:inspection}{{S115}{50}{First-passage statistics}{equation.S115}{}}
\newlabel{eq:inspection@cref}{{[equation][115][]S115}{[1][50][]50}}
\newlabel{eq:excess-returns}{{S116}{50}{First-passage statistics}{equation.S116}{}}
\newlabel{eq:excess-returns@cref}{{[equation][116][]S116}{[1][50][]50}}
\newlabel{eq:gauss-return}{{S117}{50}{First-passage statistics}{equation.S117}{}}
\newlabel{eq:gauss-return@cref}{{[equation][117][]S117}{[1][50][]50}}
\newlabel{eq:height-passage}{{S118}{51}{First-passage statistics}{equation.S118}{}}
\newlabel{eq:height-passage@cref}{{[equation][118][]S118}{[1][51][]51}}
\newlabel{si:walk-height-passage-closed}{{S119}{51}{First-passage statistics}{equation.S119}{}}
\newlabel{si:walk-height-passage-closed@cref}{{[equation][119][]S119}{[1][51][]51}}
\newlabel{si:walk-tests}{{S11.2}{51}{Numerical tests}{section*.19}{}}
\newlabel{si:walk-tests@cref}{{[subsection][2][11]S11.2}{[1][51][]51}}
\newlabel{fig:error-walk}{{S3}{52}{The error as an occupation-number fluctuation of the walk. (A)~The two sides of \cref {eq:occupation-variance} for the bins of $\Omega $, with the value $1/\pi _b-1$ of draws without memory in gray. (B)~Mean first-passage time of each bin against its memoryless value, with \cref {eq:main-memory-time} as lines. (C)~Error of \Cref {fig:tradeoff}B of the main text for the five OPES cells against \cref {eq:main-error-iid} with the first-passage times of the walk (filled; band, $\pm 25\%$) and with draws without memory (open).\relax }{figure.caption.20}{}}
\newlabel{fig:error-walk@cref}{{[figure][3][]S3}{[1][52][]52}}
\newlabel{app:temperature}{{S12}{53}{Temperature of Tempered Replicas}{section.12}{}}
\newlabel{app:temperature@cref}{{[section][12][]S12}{[1][52][]53}}
\newlabel{si:temp-continuum}{{S12.1}{53}{Continuum Limit}{subsection.12.1}{}}
\newlabel{si:temp-continuum@cref}{{[subsection][1][12]S12.1}{[1][53][]53}}
\newlabel{si:temp-heat}{{S120}{53}{Continuum Limit}{equation.S120}{}}
\newlabel{si:temp-heat@cref}{{[equation][120][]S120}{[1][53][]53}}
\newlabel{si:temp-reverse-step}{{S121}{53}{Continuum Limit}{equation.S121}{}}
\newlabel{si:temp-reverse-step@cref}{{[equation][121][]S121}{[1][53][]53}}
\newlabel{si:temp-split}{{S122}{53}{Continuum Limit}{equation.S122}{}}
\newlabel{si:temp-split@cref}{{[equation][122][]S122}{[1][53][]53}}
\newlabel{si:temp-tempered-step}{{S123}{53}{Continuum Limit}{equation.S123}{}}
\newlabel{si:temp-tempered-step@cref}{{[equation][123][]S123}{[1][53][]53}}
\newlabel{si:temp-fokker-planck}{{S124}{54}{Continuum Limit}{equation.S124}{}}
\newlabel{si:temp-fokker-planck@cref}{{[equation][124][]S124}{[1][53][]54}}
\newlabel{eq:replica-temperature}{{S125}{54}{Continuum Limit}{equation.S125}{}}
\newlabel{eq:replica-temperature@cref}{{[equation][125][]S125}{[1][54][]54}}
\newlabel{si:temp-variance-ode}{{S126}{54}{Continuum Limit}{equation.S126}{}}
\newlabel{si:temp-variance-ode@cref}{{[equation][126][]S126}{[1][54][]54}}
\newlabel{si:temp-variance-solution}{{S127}{54}{Continuum Limit}{equation.S127}{}}
\newlabel{si:temp-variance-solution@cref}{{[equation][127][]S127}{[1][54][]54}}
\newlabel{si:temp-recursion}{{S12.2}{54}{Finite-Step Sampler}{subsection.12.2}{}}
\newlabel{si:temp-recursion@cref}{{[subsection][2][12]S12.2}{[1][54][]54}}
\newlabel{si:temp-contraction}{{S128}{54}{Finite-Step Sampler}{equation.S128}{}}
\newlabel{si:temp-contraction@cref}{{[equation][128][]S128}{[1][54][]54}}
\newlabel{tab:native-temperature}{{S5}{55}{Harmonic theory on the 200-step Boltz-2 schedule. Native: terminal variance of the base sampler over the mode variance $v$, at $\eta =1.5$ (shipped) and $\eta =1$. Last column: hottest campaign replica ($m=-0.2$) over the base sampler, from \cref {eq:mode-recursion}.\relax }{table.caption.21}{}}
\newlabel{tab:native-temperature@cref}{{[table][5][]S5}{[1][55][]55}}
\newlabel{si:temp-noised}{{S129}{55}{Finite-Step Sampler}{equation.S129}{}}
\newlabel{si:temp-noised@cref}{{[equation][129][]S129}{[1][55][]55}}
\newlabel{eq:mode-recursion}{{S130}{55}{Finite-Step Sampler}{equation.S130}{}}
\newlabel{eq:mode-recursion@cref}{{[equation][130][]S130}{[1][55][]55}}
\newlabel{si:temp-trel}{{S131}{55}{Finite-Step Sampler}{equation.S131}{}}
\newlabel{si:temp-trel@cref}{{[equation][131][]S131}{[1][55][]55}}
\newlabel{si:temp-noise-only}{{S132}{55}{Finite-Step Sampler}{equation.S132}{}}
\newlabel{si:temp-noise-only@cref}{{[equation][132][]S132}{[1][55][]55}}
\newlabel{si:temp-thermometers}{{S12.3}{56}{Stein Thermometers}{subsection.12.3}{}}
\newlabel{si:temp-thermometers@cref}{{[subsection][3][12]S12.3}{[1][56][]56}}
\newlabel{si:temp-divergence}{{S133}{56}{Stein Thermometers}{equation.S133}{}}
\newlabel{si:temp-divergence@cref}{{[equation][133][]S133}{[1][56][]56}}
\newlabel{eq:stein-thermometer}{{S134}{56}{Stein Thermometers}{equation.S134}{}}
\newlabel{eq:stein-thermometer@cref}{{[equation][134][]S134}{[1][56][]56}}
\newlabel{si:temp-tconf}{{S12.4}{56}{Configurational Temperature}{subsection.12.4}{}}
\newlabel{si:temp-tconf@cref}{{[subsection][4][12]S12.4}{[1][56][]56}}
\newlabel{fig:temperature}{{S4}{57}{Temperature along the composite ladders. Left, temperature of each replica of MAP2K1 Composite Explore relative to replica~$0$, with the target of the tilt, the noise-shell measurement and the harmonic theory of \cref {eq:mode-recursion} for a soft and a stiff mode. Right, AMARO configurational temperature of replica~$0$ and of seven bands of hotter replicas with 16--84\% bootstrap ranges, where color marks the target and line style marks the method.\relax }{figure.caption.22}{}}
\newlabel{fig:temperature@cref}{{[figure][4][]S4}{[1][56][]57}}
\newlabel{eq:tconf}{{S135}{57}{Configurational Temperature}{equation.S135}{}}
\newlabel{eq:tconf@cref}{{[equation][135][]S135}{[1][56][]57}}
\newlabel{si:temp-hvp}{{S136}{57}{Configurational Temperature}{equation.S136}{}}
\newlabel{si:temp-hvp@cref}{{[equation][136][]S136}{[1][57][]57}}
\newlabel{sec:pilot}{{S12.5}{58}{Choice of Tempering}{subsection.12.5}{}}
\newlabel{sec:pilot@cref}{{[subsection][5][12]S12.5}{[1][58][]58}}
\newlabel{si:temp-cases}{{S12.6}{58}{Temperature of the Case Studies}{subsection.12.6}{}}
\newlabel{si:temp-cases@cref}{{[subsection][6][12]S12.6}{[1][58][]58}}
\newlabel{fig:evaluations}{{S5}{59}{Equilibrium statistics of the case studies. (A)~AMARO temperature of replica~$0$ and of the hottest band of the ladder for six cells against the $320$--$450$~K training range of the potential (shaded; \Cref {tab:temperature}). (B)~Measured equilibria (\Cref {tab:equilibria}), with the measured penalty of each state (blue; a bar spans two measurements, an arrow is a bound), the model's probability of the region containing the state (ochre, an upper bound) and the model's own rare state with its $F_\theta $ (purple).\relax }{figure.caption.23}{}}
\newlabel{fig:evaluations@cref}{{[figure][5][]S5}{[1][58][]59}}
\newlabel{fig:equilibrium}{{S5}{59}{Equilibrium statistics of the case studies. (A)~AMARO temperature of replica~$0$ and of the hottest band of the ladder for six cells against the $320$--$450$~K training range of the potential (shaded; \Cref {tab:temperature}). (B)~Measured equilibria (\Cref {tab:equilibria}), with the measured penalty of each state (blue; a bar spans two measurements, an arrow is a bound), the model's probability of the region containing the state (ochre, an upper bound) and the model's own rare state with its $F_\theta $ (purple).\relax }{figure.caption.23}{}}
\newlabel{fig:equilibrium@cref}{{[figure][5][]S5}{[1][58][]59}}
\newlabel{tab:temperature}{{S6}{59}{Temperature of the composite cells: relative temperature of the hottest replica (target and measured noise shell) and AMARO configurational temperature of replica~$0$ and of the hottest band, with 16--84\% bootstrap ranges, for the six cells with AMARO measurements.\relax }{table.caption.24}{}}
\newlabel{tab:temperature@cref}{{[table][6][]S6}{[1][58][]59}}
\newlabel{app:supporting}{{S13}{59}{Supplementary Results}{section.13}{}}
\newlabel{app:supporting@cref}{{[section][13][]S13}{[1][59][]59}}
\newlabel{si:res-chignolin}{{S13}{60}{Misfolded hairpin of chignolin}{section*.25}{}}
\newlabel{si:res-chignolin@cref}{{[section][13][]S13}{[1][60][]60}}
\newlabel{fig:chignolin-ring}{{S6}{61}{Chignolin with the ring distance as a coordinate. For each biased method, $F_\theta $ on the Asp3~N--Gly7~O distance and the distance between the centroids of the Tyr2 and Trp9 rings, for the samples with an Asp3~N--Thr8~O distance of $5.5$--$7.5$~\AA , the strip that holds state~\stmark {2} and the misfolded hairpin m. Each surface is zero at the minimum of state~\stmark {2}. Dashed, the basin of m up to its pass or to $3$ above its minimum; $\ddagger $, the highest point of the lowest pass between the two minima; white dots, the independent draws of the strip. Under each panel, the height of m above state~\stmark {2} and of the pass above m. Right, AMARO energy of the scored structures of the strip relative to state~\stmark {1} against the ring distance (points), with the median and interquartile range.\relax }{figure.caption.26}{}}
\newlabel{fig:chignolin-ring@cref}{{[figure][6][]S6}{[1][60][]61}}
\newlabel{si:res-equilibria}{{S13}{61}{Comparison with measured equilibria}{section*.27}{}}
\newlabel{si:res-equilibria@cref}{{[section][13][]S13}{[1][61][]61}}
\newlabel{si:res-two-state}{{S137}{62}{Chignolin folding}{equation.S137}{}}
\newlabel{si:res-two-state@cref}{{[equation][137][]S137}{[1][62][]62}}
\newlabel{si:res-cycle}{{S138}{62}{Src clamp release}{equation.S138}{}}
\newlabel{si:res-cycle@cref}{{[equation][138][]S138}{[1][62][]62}}
\newlabel{tab:equilibria}{{S7}{63}{Measured equilibria against the model (\Cref {fig:evaluations}B). The measured column gives the penalty of the state in $k_{\mathrm B}T$, or a bound. The region columns give the model's probability of the region that contains the state and $-\ln $ of that probability, which is an upper bound on the population of any state inside the region (counting uncertainty $1/\sqrt {n}$). The last column gives the model's resolved rare state on the same input and its $F_\theta $ relative to the dominant state on the independent estimate. Constructs and conditions are those of the text.\relax }{table.caption.31}{}}
\newlabel{tab:equilibria@cref}{{[table][7][]S7}{[1][63][]63}}
\newlabel{si:res-mapping}{{S13}{63}{Structures from adiabatic mapping}{section*.32}{}}
\newlabel{si:res-mapping@cref}{{[section][13][]S13}{[1][63][]63}}
\newlabel{si:res-training}{{S13}{64}{Training counterparts of sampled states}{section*.34}{}}
\newlabel{si:res-training@cref}{{[section][13][]S13}{[1][64][]64}}
\newlabel{fig:drag-structures}{{S7}{65}{Minimized structures against the model's structures along the strings of chignolin, MAP2K1--FZC and EF-Tu with GDP (ff14SB/GAFF; \Cref {app:string-drag}). Top, the RMSD of the moving part between minimized and model structures at the same string point (orange) and among the model's structures there (purple), medians over pairs, after superposing the C$\alpha $ atoms of the other residues; titles give the size of the moving part and its shift in the model between the first and last point. Bottom, the displacement of the moving part projected on the model's own change, $0$ at the first state of the model and $1$ at its last, for the model's structures (purple) and the minimized structures (blue). Points with fewer than three model structures within four grid bins are left empty.\relax }{figure.caption.33}{}}
\newlabel{fig:drag-structures@cref}{{[figure][7][]S7}{[1][64][]65}}
\newlabel{tab:experiment}{{S8}{66}{Each state of the model against experiment and the training set. Distances are C$\alpha $ RMSD of the element compared after superposing the core (medians over i.i.d.\ structures), or ligand RMSD for poses; training entries are those released before 1~June~2023. ``Memorized'': a training structure reproduces the state; ``recombined'': each part has a training counterpart but no single entry has them together; ``new'': no close training counterpart.\relax }{table.caption.35}{}}
\newlabel{tab:experiment@cref}{{[table][8][]S8}{[1][66][]66}}
\newlabel{si:res-mek1}{{S13}{67}{Second pose of MAP2K1}{section*.36}{}}
\newlabel{si:res-mek1@cref}{{[section][13][]S13}{[1][66][]67}}
\newlabel{si:res-p38}{{S13}{67}{Flexibility of \texorpdfstring {p38$\alpha $}{p38 alpha}}{section*.38}{}}
\newlabel{si:res-p38@cref}{{[section][13][]S13}{[1][67][]67}}
\newlabel{fig:mek1-amine-sites}{{S8}{68}{Polar atoms of training ligands at the two amine sites of MAP2K1--FZC, in the pocket of state~\stmark {2} of the model, seen down the normal of the plane of the two aminocyclohexyl rings. FZC of state~\stmark {1} (gray) and of state~\stmark {2} (gold) with their amine nitrogens (spheres), and the four polar residues of the pocket (green sticks, named beside A). (A)~MEK1 training structures, with DS94070624 of 7XNC (blue) and the ribose O3$'$ of nucleotides (red, $83$ ligands). (B)~Amine nitrogens of inhibitors bound to other kinases (violet, $409$ atoms). Training atoms are shown within $2\,\text {\AA }$ of the ring plane and $4\,\text {\AA }$ of either amine.\relax }{figure.caption.37}{}}
\newlabel{fig:mek1-amine-sites@cref}{{[figure][8][]S8}{[1][67][]68}}
\newlabel{fig:p38-rmsf}{{S9}{69}{Per-residue C$\alpha $ displacement between lipid-closed 1A9U and lipid-open 3HVC (black) and the model's C$\alpha $ RMSF (blue) for (A)~4-FPP alone and (B)~SB203580 plus 4-FPP, after C-lobe core superposition (\Cref {app:experiment}). The lipid-pocket segments (UniProt $189$--$202$, $230$--$262$, $289$--$298$) are shaded; Gly170 and the lid residues Trp197 and Met198 are marked. The $\alpha \text {1L}/\alpha \text {2L}$ motion at residues $240$--$260$ is absent from the RMSF.\relax }{figure.caption.39}{}}
\newlabel{fig:p38-rmsf@cref}{{[figure][9][]S9}{[1][68][]69}}
